# Supplementary material for: Learnable Spatial-Temporal Positional Encoding for Link Prediction
Source: arXiv:2506.08309 source file (2025-06-11)
Supplement: Supplementary file 1 [file main_appendix.tex]

% \input{tables/auc_roc_transductive}

% \input{tables/ap_inductive}

% \input{tables/auc_roc_inductive}
